# Supplementary material for: Deep Reinforcement Learning for Conservation Decisions
Source: arXiv:2106.08272 source file (2021-06-15)
Supplement: Supplementary file 1 [file appendix-A-definitions.pdf]

# Appendix A: Deep Reinforcement Learning

A Preprint

**Marcus Lapeyrolerie**
Department of Environmental Science, Policy, and Management
University of California, Berkeley
Berkeley, California

**Melissa Chapman**
Department of Environmental Science, Policy, and Management
University of California, Berkeley
Berkeley, California

**Kari Norman**
Department of Environmental Science, Policy, and Management
University of California, Berkeley
Berkeley, California

**Carl Boettiger**
Department of Environmental Science, Policy, and Management
University of California, Berkeley
Berkeley, California
cboettig@berkeley.edu

June 14, 2021

***K*eywords** Decision Theory · Conservation · Artificial Intelligence · Machine Learning · Tipping Points · Fisheries

In this appendix, we will go into further detail on how deep RL algorithms work. The aim here is not to give full treatment of all deep RL methods; instead, this section is meant to serve as an abbreviated background view on model-free deep RL[1]. We will introduce some of the important design choices that are made for model-free deep RL algorithms and will point to specific resources that give a more complete presentation. These sections presume some familiarity with gradient descent optimization – see Ruder (2017) for a thorough treatment. Throughout these sections, we'll consider the environment to be an MDP which makes for a cleaner presentation and is also consistent with the referenced literature. This treatment can be extended to the POMDP case by including observations and the emission function.

[1]We focus on model-free methods because the agents we use in the manuscript and Appendix B are all model-free. Further, model-based algorithms generalize from the methods we discuss here except model-based agents attempt to learn or use the environment's state-transition operator, which is typically used for planning or supplementary sample generation (Sutton and Barto 2018).

# 1 Gradient-based Model-free RL Algorithms

Among model-free methods, there is divergence around what functions the agent is attempting to learn in order to achieve the RL objective. Generally, model-free agents either learn a policy function, a value function or both. For context, *value functions* are proxies for how high of a cumulative reward an agent can expect to receive from a given state or state-action pair. If an agent knows the value function, then the agent can find the optimal action at any state by selecting the action that will maximize the value function in expectation. The class of algorithms that exclusively tries to learn a value function are called *value-based* methods. In contrast, *policy gradient* algorithms exclusively learn the policy. And, lastly, *actor-critic* algorithms attempt to learn both a policy and value function, whereby the value function is used to inform the agent on the goodness of a selected action. We will go into further detail on these different approaches below.

## 1.1 Policy Gradients

The most straightforward way to optimize the RL objective is through a policy search, whereby the agent continually updates its policy to maximize rewards. In deep RL, the agent's policy, $\pi$, is parameterized by a neural network. The parameters of the policy neural network are commonly denoted by $\theta$. In policy gradient methods, the RL agent performs gradient ascent on the expected return, $J(\pi_\theta)$, to find the optimal policy parameters. At each gradient step, which we'll index using $k$, the following update is performed,

$$\theta_{k+1} = \theta_k + \alpha \nabla_{\theta_k} J(\pi_{\theta_k}).$$

Supposing that the agent has interacted with the environment and has collected some trajectories denoted by, $\tau_i$, we can employ the policy gradient theorem – see Sutton and Barto (2018) for the proof of the policy gradient theorem – to estimate $\nabla J(\pi_\theta)$ as:

$$\nabla_\theta J(\pi_\theta) \approx \sum_{i,t} \nabla_\theta \log \pi_\theta(a_{i,t} \mid s_{i,t}) \Big( \sum_{t'=t}^{H} \gamma^{t'-t} r(s_{i,t'}, a_{i,t'}) \Big).$$

The intuition behind this approximation is exactly what we want: the agent will increase the probability of repeating the actions for the inputted states proportional to the size of the return. In practice, however, the empirical return tends to have high variance, resulting in very noisy gradients that impede learning (Sutton and Barto 2018). To avoid this issue, many policy gradient algorithms replace the empirical return with a return estimator that has lower variance (Sutton and Barto 2018).

A sketch of a simple policy gradient algorithm is shown in Algorithm 1[2].[3]

**Algorithm 1** Generic On-policy Policy Gradient Algorithm

Input initial policy parameters $\theta_0$
**for** $k = 0, 1, 2, \ldots$ **do**
    Generate a trajectory $\{s_i, a_i, r_i\}$ by following an exploration algorithm with the policy $\pi_{\theta_k}$ (e.g. $\epsilon$-greedy)
    **for** $t = 0, 1, \ldots, T-1$ **do**
        $G \leftarrow \sum_{j=t}^{T-1} \gamma^{j-t} r_j$
        $\theta_{k+1} \leftarrow \theta_k + \alpha \gamma^t G \, \nabla_{\theta_k} \log \pi_{\theta_k}(a_t|s_t)$

## 1.2 Value-based Methods

Another way to approach the RL problem is by estimating a value function, and then using the value function to retrieve a policy. Value functions attempt to quantify the goodness of being in a state or taking an action from a state. Given that the objective of RL is to maximize the cumulative reward, "goodness" refers to

[2]The algorithm sketches showed throughout this study are not practical for a variety of reasons including high bias estimators, high variance estimators and correlated samples. The algorithm examples are instead intended to convey how the general steps of the different algorithm classes come together.

[3]In this algorithm, we mention exploration algorithms which we discuss later in Section 2.

how high of a cumulative reward the agent can expect to receive. For example, the state-action-value or Q function finds the expected return from a state-action pair under a policy, $\pi$,

$$Q^{\pi}(s_t, a_t) = \mathbb{E}_{\tau \sim p_{\pi}(\tau|s_t,a_t)}\left[\sum_{t'=t}^{H} \gamma^{t'-t} r(s_t, a_t)\right].$$

There are more value functions that can used in practice (Schulman et al. 2018), but since Q-functions are commonly encountered, we will focus on Q-learning. From the above equation, we can also define the Q function recursively,

$$Q^{\pi}(s_t, a_t) = r(s_t, a_t) + \gamma\, \mathbb{E}_{s_{t+1} \sim T(s_{t+1}|s_t,a_t),\, a_{t+1} \sim \pi(a_{t+1}|s_{t+1})}\left[Q^{\pi}(s_{t+1}, a_{t+1})\right].$$

The motivation behind Q-learning is that if we know the Q function under certain conditions – e.g. that the state-action space is discrete and that all state-action pairs are visited ad infinitum[4] (Sutton and Barto 2018, 131; Melo, n.d.) –, then we can easily find the optimal action at any state by selecting the action with the highest Q-value: $a_t^* = \underset{a_t}{\operatorname{argmax}}\, Q(s_t, a_t)$. Using this optimal policy, we can write an equation for the optimal Q-function from the recursive definition,

$$Q^{*}(s_t, a_t) = r(s_t, a_t) + \gamma\, \mathbb{E}_{s_{t+1} \sim T(s_{t+1}|s_t,a_t)}\left[\max_{a_{t+1}} Q^{*}(s_{t+1}, a_{t+1})\right].$$

The objective for deep Q-learning is to find an approximate Q-function that satisfies the above equation, where we represent our approximate Q-function, $Q_\phi$, with a neural network that has the parameters of $\phi$. Subtracting the left hand and right hand side of the recursive Q-function definition, we can define the temporal difference (TD) error, $\mathcal{E}$, for a state-action pair as

$$\mathcal{E} = r(s_t, a_t) + \gamma \max_{a} Q_\phi(s_{t+1}, a) - Q_\phi(s_t, a_t).$$

The goal is to find a $Q_\phi$ that sets the TD error to zero across all state-action pairs. The general process to achieve this objective is to sample trajectories from the environment, evaluate the TD Error across different state-action-reward transitions – with samples indexed by $i$ –, and then perform the following gradient descent on the parameters of the Q-function neural network:

$$\phi_{k+1} = \phi_k - \alpha \nabla_{\phi_k} \sum_i \mathcal{E}_i^2.$$

After the Q-function neural network or Q-network has been fitted, the agent will select actions by inputting the current state into the Q network and then identifying the state-action pair with the highest approximated Q value. The benefit of using neural networks to approximate Q-functions is that neural networks are able to generalize Q functions to unseen state-action pairs, whereas classic methods like TD-learning are not able to generalize (Mnih et al. 2015). But there a host of problems with getting neural-network-based value-learning agents to work in practice; see Mnih et al. (2015) and Hasselt, Guez, and Silver (2015) for more insight on these issues.

A notable concern with these methods is that they tend to suffer from bias which is introduced by fitting a value network to a target that incorporates an estimated value function (Hasselt, Guez, and Silver 2015). In review, a sketch of a simple deep Q learning algorithm is shown in Algorithm 2.

### 1.3 Actor-Critic

Actor-critic algorithms integrate the main components from both value-learning and policy gradient based methods. The "actor" attempts to learn the policy, and the "critic" attempts to learn a value function. While the general algorithm for the critic is exactly the same as mentioned in the value-learning section, the actor differs from policy gradient algorithms by incorporating the critic in its gradient ascent step. The gradient of the return is estimated as

[4]These conditions are of course rarely true, but approximate Q-learning has still been able to achieve notable successes (Mnih et al. 2015).

**Algorithm 2** Generic On-policy Q-learning Algorithm

Input initial Q-network parameters $\phi_0$
**for** $k = 0, 1, 2, \ldots$ **do**
  **for** $t = 0, 1, \ldots, T-1$ **do**
    Select an action $a_t$ using $Q_{\phi_k}$ according to an exploration algorithm (e.g. $\epsilon$-greedy)
    Take action $a_t$ and observe $r_t, s_{t+1}$
    $\mathcal{E} \leftarrow r_t + \gamma \max_a Q_{\phi_k}(s_{t+1}, a) - Q_{\phi_k}(s_t, a_t)$
    $\phi_{k+1} \leftarrow \phi_k - \alpha \nabla_{\phi_k} \mathcal{E}^2$

$$\nabla_\theta J(\pi_\theta) \approx \sum_{i,t} \nabla_\theta \log \pi_\theta(a_{i,t} \mid s_{i,t}) \, \hat{Q}(s_{i,t}, a_{i,t}).$$

where $\hat{Q}$ is a value function estimated by the critic. The benefit of actor-critic algorithms is that they can balance the issues with bias and variance that are common with value-learning and policy gradient methods respectively (Sutton and Barto 2018). Consequently, actor-critic algorithms have achieved many of the state of the art results in model-free deep RL (Haarnoja et al. 2018; Fujimoto, Hoof, and Meger 2018).
A simple sketch of an actor-critic algorithm is shown in Algorithm 3.

**Algorithm 3** Generic On-policy Actor-Critic Algorithm

Input initial policy and Q-network parameters $\theta_0, \phi_0$
**for** $k = 0, 1, 2, \ldots$ **do**
  Generate a trajectory $\{s_i, a_i, r_i\}$ by following an exploration algorithm with the policy $\pi_k$ (e.g. $\epsilon$-greedy)
  **for** $t = 0, 1, \ldots, T-1$ **do**
    $\mathcal{E} \leftarrow r_t + \gamma \max_a Q_{\phi_k}(s_{t+1}, a) - Q_{\phi_k}(s_t, a_t)$
    $\phi_{k+1} \leftarrow \phi_k - \alpha \nabla_{\phi_k} \mathcal{E}^2$
    $\theta_{k+1} \leftarrow \theta_k + \alpha \, \nabla_{\theta_k} \log \pi_{\theta_k}(a_t|s_t) Q_{\phi_k}(s_t, a_t)$

## 2 Exploration

Over the course of training, RL agents will engage in trial and error learning, whereby it will be necessary for the agent to explore new sequences of actions as well as exploit past high rewarding sequences. In the sections above, we procedurally mentioned that the agent must select actions during training. Yet, how the agent selects these actions is very important because if an agent explores the state-action space poorly, the agent will learn a sub-optimal policy. The fundamental issue is that it is very difficult for the agent to know when it should engage in explorative or exploitative behavior. This *exploration-exploitation dilemma* is an open research question (Berger-Tal et al. 2014). For RL problems with small state-action spaces, e.g. space-action spaces that can be represented in a table, simple exploration algorithms will converge to the optimal policy, but with large or infinite state-action spaces, there are no convergence guarantees (Berger-Tal et al. 2014).

Current deep RL algorithms take a range of approaches towards this dilemma. In the sections below, we will present some of the more commonly encountered exploration algorithms and then point to some more advanced methods.

### 2.1 Epsilon-Greedy Algorithm

The Epsilon-Greedy algorithm takes a very simple approach towards balancing exploration and exploitation. For some $\epsilon \in (0, 1)$, an Epsilon-Greedy agent exploits the best available action with probability $1 - \epsilon$ and explores a random action with probability $\epsilon$. While simplistic, this algorithm has been effective on a range of problems (Mnih et al. 2015).

### 2.2 Boltzmann Exploration

For algorithms that learn a value function, agents can select actions by sampling from a Boltzmann or Softmax distribution that is constructed over the value function. So if the agent is doing Q-learning, the probability for the agent to select the action, $a$, would be:

$$P(a) = \frac{e^{\frac{Q(s_t,a)}{\tau}}}{\sum_{a'} e^{\frac{Q(s_t,a')}{\tau}}}$$

where $\tau \in (0, \infty)$ is called the temperature parameter and controls how much the agent will weight high Q scores over low Q scores. The advantage of using Boltzmann exploration is that since the probability of selecting an action is proportional to how good the agent thinks that action is, the agent can explore the space more efficiently than with Epsilon-Greedy exploration.

### 2.3 Noise-Based Exploration

Injecting noise into an agent's action, observation or parameter space is another simple yet effective exploration method. With noise addition, there are a number of design choices that can be made. For instance, noise can be sampled from different distributions (Plappert et al. 2018), scaled adaptively based on the policy(Plappert et al. 2018), or sampled according to the state that the agent observes (Raffin and Stulp 2020). There are a variety of reasons why one would want to use each of these variations; these reasons are well discussed in Plappert et al. (2018) and Raffin and Stulp (2020).

### 2.4 Entropy-based Exploration

An increasingly common way to achieve exploration is by adding a function of the entropy term, $H(\pi(a|s))$, to the loss function of the policy network. By adding this term, the agent has an incentive to learn a policy that balances reward-seeking and explorative behavior. While this introduces some bias as the agent no longer exclusively maximizes cumulative rewards, entropy-based exploration has achieved state of the art results (Haarnoja et al. 2018). For more, Ahmed et al. (2019) gives a thorough discussion on the benefits of using entropy.

### 2.5 More Advanced Exploration Methods

There is a multitude of exploration algorithms that we have not touched on. It is important to note that the algorithms mentioned above are generally suited for dense reward or "easy-exploration" problems. "Hard-exploration" problems, like a maze environment which has very few state-action pairs with significant rewards, often require more intricate and bespoke exploration algorithms. The issue for "hard-exploration" problems is that the agent needs to explore the state-action space efficiently, and simple exploration algorithms will waste computational time by revisiting bad actions. Two common approaches to hard exploration problems are memory-based and curiosity-driven techniques. For the sake of brevity, we will not go into further detail on these approaches but will provide some promising recent work. Look at Ecoffet et al. (2021) and Badia et al. (2020) for recent applications of memory-based exploration. See Burda et al. (2018) and Bellemare et al. (2016) for recent studies of curiosity-driven methods.

## 3 On-Policy vs. Off-policy Evaluation

Before deciding how to explore the environment, RL algorithms must have a policy to use during training. RL agents can either select actions from the same policy that they intend to use during evaluation or they can sample actions from a policy that is different. The former is called *on-policy* learning: the on-policy agent learns to select actions with the same policy it will use in testing. The latter is called *off-policy* learning: the off-policy agent uses a policy during training that is potentially different than the policy that the agent will evaluate.

A significant issue that arises when agents learn from their experience is correlation of samples (Mnih et al. 2015; Schaul et al. 2016). In the simple case that we have an RL agent that interacts with the environment for a few time steps and then uses this trajectory for its learning update, these samples, since they come from the same trajectory, will be strongly correlated (Mnih et al. 2015). Learning from correlated samples

is undesirable since this can result in agents getting stuck in local optima, which will impede learning, but there are other reasons why learning from a single trajectory causes problems – see Schaul et al. (2016) and Mnih et al. (2015) for more insight here.

On-policy and off-policy agents have different solutions to the correlated samples problem. If the agent is off-policy, the agent can employ a replay buffer – see Mnih et al. (2015) for an example of a replay buffer-based agent. With a replay buffer, the agent saves state-action-reward transitions in the replay buffer, and during learning updates, the agent samples transitions from the buffer. Since the replay buffer can be arbitrarily large and thus store transitions from numerous trajectories, sampling from the buffer results in decorrelated samples. On-policy agents, however, cannot use a replay buffer since these agents are not allowed to use samples from a policy different than the policy they are trying to improve – n.b. replay buffers are generally large enough to hold transitions from multiple policies. The solution to de-correlate samples for on-policy agents is to use parallel workers, whereby multiple workers explore the environment according to the current policy. Due to stochasticity that can come from exploration and the environment, the workers go on different trajectories in state-action space. The agent will collect samples across these workers in a learning step, perform its learning step and then repeat the process of collecting and sampling transitions with an updated policy. The idea behind using parallel workers is that sampling over multiple trajectories de-correlates samples – see Babaeizadeh et al. (2017) on more details here. In practice, using a large replay buffer, on the order of millions of transitions, or a modest number of parallel, around 4-16 for simple RL problems, is very important to achieve good agent performance.

## 4 Next Steps

Reinforcement learning is a huge, constantly evolving field, and we've only touched on a small sliver of RL in our study. In this appendix, we briefly introduced some of the major design decisions that are made with model-free deep RL algorithms, but there are many more decisions that are made with state of the art model-free agents. In Table 1, we collect some of the more commonly used model-free deep RL algorithms. Readers who are interested in learning more about the current state of deep RL should read the literature referenced in Table 1; Mnih et al. (2015), Haarnoja et al. (2018) and Schulman, Wolski, et al. (2017) are good places to start. It is important to note that while we have focused on gradient-based, model-free methods, there has also been promising recent development with model-based and gradient-free techniques. See Janner et al. (2019) and Weber et al. (2018) for recent examples of model-based deep RL algorithms, and Salimans et al. (2017) as a recent example of a gradient-free approach. A benefit of model-free deep RL over these other methods is that there has been more of a general focus on model-free deep RL, so there are widely available software packages like Stable Baselines and TensorFlow Agents which implement model-free deep RL agents. However, it is important to keep in mind though that deep RL has only become established in the last decade, and with the large amount of open research questions, deep RL may evolve significantly in the near future.

| Abbreviation | Algorithm Name | Policy | Method |
|---|---|---|---|
| A2C | Advantage Actor Critic (Mnih et al. 2016) | On-policy | Actor-critic |
| A3C | Asynchronous A2C (Babaeizadeh et al. 2017) | On-policy | Actor-critic |
| TRPO | Trust Region Policy Optimization (Schulman, Levine,et al. 2017) | On-policy | Policy Gradient |
| PPO | Proximal Policy Optimization (Schulman, Wolski, et al. 2017) | On-policy | Actor-critic |
| DQN | Deep Q Networks (Mnih et al. 2015) | Off-policy | Value-Based |
| DDPG | Deep Deterministic Policy Gradient (Lillicrap et al. 2019) | Off-policy | Actor-critic |
| TD3 | Twin Delayed DDPG (Fujimoto, Hoof, and Meger 2018) | Off-policy | Actor-critic |
| SAC | Soft Actor Critic (Haarnoja et al. 2018) | Off-policy | Actor-critic |
| IMPALA | Importance Weighted Actor Learner (Espeholt et al. 2018) | Off-policy | Actor-critic |

Table 1: Survey of common model-free deep RL algorithms.

## References

Ahmed, Zafarali, Nicolas Le Roux, Mohammad Norouzi, and Dale Schuurmans. 2019. "Understanding the Impact of Entropy on Policy Optimization." *arXiv:1811.11214 [Cs, Stat]*, June. http://arxiv.org/abs/1811.11214.

Babaeizadeh, Mohammad, Iuri Frosio, Stephen Tyree, Jason Clemons, and Jan Kautz. 2017. "Reinforcement Learning Through Asynchronous Advantage Actor-Critic on a GPU." *arXiv:1611.06256 [Cs]*, March. http://arxiv.org/abs/1611.06256.

Badia, Adrià Puigdomènech, Pablo Sprechmann, Alex Vitvitskyi, Daniel Guo, Bilal Piot, Steven Kapturowski, Olivier Tieleman, et al. 2020. "Never Give Up: Learning Directed Exploration Strategies." *arXiv:2002.06038 [Cs, Stat]*, February. http://arxiv.org/abs/2002.06038.

Bellemare, Marc G., Sriram Srinivasan, Georg Ostrovski, Tom Schaul, David Saxton, and Remi Munos. 2016. "Unifying Count-Based Exploration and Intrinsic Motivation." *arXiv:1606.01868 [Cs, Stat]*, November. http://arxiv.org/abs/1606.01868.

Berger-Tal, Oded, Jonathan Nathan, Ehud Meron, and David Saltz. 2014. "The Exploration-Exploitation Dilemma: A Multidisciplinary Framework." *PLOS ONE* 9 (4): e95693. https://doi.org/10.1371/journal.pone.0095693.

Burda, Yuri, Harri Edwards, Deepak Pathak, Amos Storkey, Trevor Darrell, and Alexei A. Efros. 2018. "Large-Scale Study of Curiosity-Driven Learning." *arXiv:1808.04355 [Cs, Stat]*, August. http://arxiv.org/abs/1808.04355.

Ecoffet, Adrien, Joost Huizinga, Joel Lehman, Kenneth O. Stanley, and Jeff Clune. 2021. "Go-Explore: A New Approach for Hard-Exploration Problems." *arXiv:1901.10995 [Cs, Stat]*, February. http://arxiv.org/abs/1901.10995.

Espeholt, Lasse, Hubert Soyer, Remi Munos, Karen Simonyan, Volodymir Mnih, Tom Ward, Yotam Doron, et al. 2018. "IMPALA: Scalable Distributed Deep-RL with Importance Weighted Actor-Learner Architectures." *arXiv:1802.01561 [Cs]*, June. http://arxiv.org/abs/1802.01561.

Fujimoto, Scott, Herke van Hoof, and David Meger. 2018. "Addressing Function Approximation Error in Actor-Critic Methods." *arXiv:1802.09477 [Cs, Stat]*, October. http://arxiv.org/abs/1802.09477.

Haarnoja, Tuomas, Aurick Zhou, Pieter Abbeel, and Sergey Levine. 2018. "Soft Actor-Critic: Off-Policy Maximum Entropy Deep Reinforcement Learning with a Stochastic Actor." *arXiv:1801.01290 [Cs, Stat]*, August. http://arxiv.org/abs/1801.01290.

Hasselt, Hado van, Arthur Guez, and David Silver. 2015. "Deep Reinforcement Learning with Double Q-Learning." *arXiv:1509.06461 [Cs]*, December. http://arxiv.org/abs/1509.06461.

Janner, Michael, Justin Fu, Marvin Zhang, and Sergey Levine. 2019. "When to Trust Your Model: Model-Based Policy Optimization." *arXiv:1906.08253 [Cs, Stat]*, November. http://arxiv.org/abs/1906.08253.

Lillicrap, Timothy P., Jonathan J. Hunt, Alexander Pritzel, Nicolas Heess, Tom Erez, Yuval Tassa, David Silver, and Daan Wierstra. 2019. "Continuous Control with Deep Reinforcement Learning." *arXiv:1509.02971 [Cs, Stat]*, July. http://arxiv.org/abs/1509.02971.

Melo, Francisco S. n.d. "Convergence of Q-Learning: A Simple Proof," 4.

Mnih, Volodymyr, Adrià Puigdomènech Badia, Mehdi Mirza, Alex Graves, Timothy P. Lillicrap, Tim Harley, David Silver, and Koray Kavukcuoglu. 2016. "Asynchronous Methods for Deep Reinforcement Learning." *arXiv:1602.01783 [Cs]*, June. http://arxiv.org/abs/1602.01783.

Mnih, Volodymyr, Koray Kavukcuoglu, David Silver, Andrei A. Rusu, Joel Veness, Marc G. Bellemare, Alex Graves, et al. 2015. "Human-Level Control Through Deep Reinforcement Learning." *Nature* 518 (7540): 529–33. https://doi.org/10.1038/nature14236.

Plappert, Matthias, Rein Houthooft, Prafulla Dhariwal, Szymon Sidor, Richard Y. Chen, Xi Chen, Tamim Asfour, Pieter Abbeel, and Marcin Andrychowicz. 2018. "Parameter Space Noise for Exploration." *arXiv:1706.01905 [Cs, Stat]*, January. http://arxiv.org/abs/1706.01905.

Raffin, Antonin, and Freek Stulp. 2020. "Generalized State-Dependent Exploration for Deep Reinforcement Learning in Robotics." *arXiv:2005.05719 [Cs, Stat]*, May. http://arxiv.org/abs/2005.05719.

Ruder, Sebastian. 2017. "An Overview of Gradient Descent Optimization Algorithms." *arXiv:1609.04747 [Cs]*, June. http://arxiv.org/abs/1609.04747.

Salimans, Tim, Jonathan Ho, Xi Chen, Szymon Sidor, and Ilya Sutskever. 2017. "Evolution Strategies as a Scalable Alternative to Reinforcement Learning." *arXiv:1703.03864 [Cs, Stat]*, September. http://arxiv.org/abs/1703.03864.

Schaul, Tom, John Quan, Ioannis Antonoglou, and David Silver. 2016. "Prioritized Experience Replay." *arXiv:1511.05952 [Cs]*, February. http://arxiv.org/abs/1511.05952.

Schulman, John, Sergey Levine, Philipp Moritz, Michael I. Jordan, and Pieter Abbeel. 2017. "Trust Region Policy Optimization." *arXiv:1502.05477 [Cs]*, April. http://arxiv.org/abs/1502.05477.

Schulman, John, Philipp Moritz, Sergey Levine, Michael Jordan, and Pieter Abbeel. 2018. "High-Dimensional Continuous Control Using Generalized Advantage Estimation." *arXiv:1506.02438 [Cs]*, October. http://arxiv.org/abs/1506.02438.

Schulman, John, Filip Wolski, Prafulla Dhariwal, Alec Radford, and Oleg Klimov. 2017. "Proximal Policy Optimization Algorithms." *arXiv:1707.06347 [Cs]*, August. http://arxiv.org/abs/1707.06347.

Sutton, Richard S, and Andrew G Barto. 2018. *Reinforcement Learning: An Introduction.* MIT press.

Weber, Théophane, Sébastien Racanière, David P. Reichert, Lars Buesing, Arthur Guez, Danilo Jimenez Rezende, Adria Puigdomènech Badia, et al. 2018. "Imagination-Augmented Agents for Deep Reinforcement Learning." *arXiv:1707.06203 [Cs, Stat]*, February. http://arxiv.org/abs/1707.06203.
