# Supplementary material for: Deep Reinforcement Learning for Conservation Decisions
Source: arXiv:2106.08272 source file (2021-06-15)
Supplement: Supplementary file 2 [file appendix-B-examples.pdf]

# Appendix B: Examples of Deep RL in Ecological Decision Problems

A Preprint

**Marcus Lapeyrolerie**
Department of Environmental Science, Policy, and Management
University of California, Berkeley
Berkeley, California

**Melissa Chapman**
Department of Environmental Science, Policy, and Management
University of California, Berkeley
Berkeley, California

**Kari Norman**
Department of Environmental Science, Policy, and Management
University of California, Berkeley
Berkeley, California

**Carl Boettiger**
Department of Environmental Science, Policy, and Management
University of California, Berkeley
Berkeley, California
cboettig@berkeley.edu

June 13, 2021

## 1 Overview

In this appendix, we provide examples with annotated code illustrating how to use recent deep RL algorithms to train RL agents to make decisions in two distinct ecological management scenarios: setting a harvest quota in a fishery, and managing conservation effort in the face of ecological tipping points. The approach illustrated here should be sufficient to reproduce the results presented in the main text, and should serve as an effective starting point for researchers seeking to apply deep RL to these simulation environments, to other simulation environments we continue to develop, or to their own environments. (Appendix C details the process of defining one's own `gym` environment from an ecological model). This overview is neither a complete introduction to deep RL or a comprehensive analysis of RL solutions to these environments.

## 2 Deep Reinforcement Learning in R

Although all the necessary tooling for deep RL is most extensively implemented in Python, the R language is more familiar to most ecologists. Fortunately, modern bindings such as the `reticulate` package ("Reticulate" 2018) make it straightforward to use these tools without ever leaving the R interface. In this appendix, we detail this "pure R" approach, as well as a "pure Python" approach.

In the R based-approach, R functions take responsibility from the user for translating commands into Python code before it is executed, an approach commonly referred to as meta-programming. This still requires a local Python installation, which can be installed directly from R using the command `install_miniconda()` from the `reticulate` package in R. Alternately, users may prefer running the analysis inside a docker container. The Rocker Project ("Rocker" 2018) provides pre-built docker containers which include the necessary R and Python environments, as well as CUDA libraries required to take advantage of GPU-based acceleration on suitable architectures. This can be particularly useful for users running ML algorithms on remote servers.

By using a cache of pre-trained agents distributed with this appendix, it should be possible to efficiently reproduce the results shown here on any recent laptop with the versions of software indicated. Reproducing the training of RL agents is more computationally intensive, and a more powerful multi-core CPU or CUDA-enabled GPU is recommended. Note that hardware differences are also a source of instability in the reproduciblity of RL training (Nagarajan, Warnell, and Stone 2019).

In this appendix, we illustrate how to apply a deep reinforcement learning framework to train previously published RL algorithms on the novel decision environments as illustrated in the main text. Appendix C discusses the construction of such environments in code.

## 3 Deep Reinforcement Learning Frameworks

Rather than implement deep RL algorithms from scratch, we illustrate the use of one of the leading software frameworks for research and application of deep RL methods. At the time of writing, several major frameworks exist which provide reference implementations of the leading deep RL algorithms (see Table 1 and Appendix A). While we do not seek to provide a comprehensive review of available frameworks, some familiarity with current frameworks can be helpful. Like many machine learning libraries, these frameworks are themselves each built around one of two popular machine learning libraries, PyTorch (Paszke et al. 2019) or Tensorflow ("Tensorflow" 2018), and all are based in Python. Existing frameworks we evaluated include Keras-RL (Plappert 2016), Tensorflow Agents (Guadarrama et al. 2018), OpenAI Spinning Up (Achiam 2018) OpenAI Baselines, Stable-Baselines2 (Hill et al. 2018), and Stable-Baselines3 (Raffin et al. 2019). Keras-RL saw widespread early adoption, but is built on Tensorflow version 1.x. It is incompatible with Tensorflow 2.x and not actively maintained. Tensorflow Agents is developed by the Tensorflow team, a recent and actively developed framework with support for both Tensorflow 1.x and 2.x and good support for low-level customization of RL algorithms. However, higher-level interfaces and high-level documentation are still relatively limited. OpenAI's SpinningUp is an education-targeted framework useful for developers wanting to become more familiar with the internal methods of RL algorithms.
OpenAI's Baselines is primarily Tensorflow 1.x-based implementation of many recently published RL algorithms. Researchers at Ensta Paris Tech first created Stable Baselines as a fork of the OpenAI implementation, rigorously addressing numerous issues in documentation, testing, and coding style that have helped make their fork see even greater adoption. Stable-Baselines3 is the most recent version (Feb 2021), a ground-up rewrite which switches to a PyTorch-based implementation and further strengthens internal checks such as static types. The examples here all use the Stable-Baselines3 framework, though researchers in this area should expect frameworks to continue to emerge and evolve. Grand challenge problems will likely require significant development beyond the current algorithms and capabilities available in existing frameworks.

## 4 Getting started

Clone the repository `https://github.com/boettiger-lab/rl-intro`, e.g. using the New Project->From Version Control->Git menu in RStudio.

From the project directory, we can then install all the necessary dependencies using `renv`, which helps ensure a reproducible environment of fixed versions of R packages and Python modules.

```r
#install.packages("renv")
renv::restore()
```

```
## * The library is already synchronized with the lockfile.
## * The Python library is already up to date.
```

Python users can install the dependencies listed in the repository's `requirements.txt` and run the corresponding python scripts found in the `python/` sub-directory instead. Meanwhile, the RMarkdown source-code for this file can be found in the `appendices` directory of the project repository. Once the packages have installed, we are ready to load the necessary libraries. Note that the `import` function from `reticulate` package acts much like the `library` command in R, though it does not attach the package function to the global namespace. To make it more convenient to access those functions, we can assign a shorthand name.

```r
# R dependencies
library(tidyverse)
library(patchwork)
library(reticulate)

## Python dependencies loaded via R
sb3      = import("stable_baselines3")
torch    = import("torch")
gym      = import("gym")
gym_fishing = import("gym_fishing")
gym_conservation = import("gym_conservation")


source("../R/plotting-helpers.R")
```

Numerical reproducibility can be challenging in machine learning problems, particularly when using GPU-based acceleration (Nagarajan, Warnell, and Stone 2019). In addition to setting a random seed in our Python environment, we can optionally disable GPU use to improve reproducibility by setting the `CUDA_VISIBLE_DEVICES` to a blank value.

```r
## reproducible settings
np = import("numpy")
seed = 24L # integer
np$random$seed(seed)

# Optionally set to "" to force CPU-evaluation if needing perfect reproducibility
#Sys.setenv("CUDA_VISIBLE_DEVICES"="")
set.seed(seed)
```

The above code also illustrates a few conventions which may be helpful to bear in mind when using the `reticulate` interface to interact with Python from R: it is often necessary for integer values to be explicitly typed as integers by adding a trailing `L` (corresponding to the primitive C type `long` integer). Python is also more strongly object-oriented than many R packages, where "methods" of an "object" are accessed with the list-subset operator `$` in R (equivalent to the use of `.` in Python). Lastly, while R can use `<-` or `=` for assignment, Python uses only `=`. For simplicity we will stick with the latter.
With few exceptions, the R code shown here can be re-written as python code by dropping the `L` and replacing `$` with `.`, see stand-alone python code in the `python/` subdirectory of the repository.

# 5 Finding a known optimal solution using RL

## 5.1 Sustainable Harvest Quotas

We begin by selecting an environment from `gym_fishing`. While we use default parameter values for this example, note that is possible to pass alternative parameterizations using additional optional arguments.

```
## initialize the environment
env = gym$make("fishing-v1", sigma=0.1)
```

### 5.2 An optimal solution

Recall that under the assumptions of the simple model used in the `fishing-v1` environment, we can determine the optimal harvest policy analytically if the model and parameters are known precisely (Reed 1979). The optimal strategy is a policy of 'constant escapement,' designed to keep the remaining stock size (the population that 'escapes' fishing harvest) at the biomass corresponding to a maximum growth rate, i.e. at $B_{MSY} = K/2$ in this model. `gym_fishing` defines a collection of non-RL agents in the `models` submodule, including the a human agent that merely asks to enter their desired quota manually. The `escapement` model implements the provably optimal constant escapement rule. A third model, `msy`, implements a policy based on "Maximum Sustainable Yield" policy (Schaefer 1954), which is actually more commonly used as a basis for management than constant escapement, despite only being optimal at the steady state under deterministic dynamics.

```
# Simulate under the optimal solution (given the model)
opt = gym_fishing$models$escapement(env)
```

Note that the `escapement` function makes very specific assumptions about the environment that it is given. In particular, it assumes we can compute $B_{MSY}$ directly from the internal model of stock recruitment contained in the environment. In contrast, the RL methods make no such assumption of being able to access that internal model directly.

```
opt_sims = env$simulate(opt, reps = 100L)
opt_policy = env$policyfn(opt)
```

We can plot the resulting data.frames using standard `ggplot2` methods shown in the `R/plotting-helpers.R`, or in python using either the `plot` methods defined in `gym_fishing` or standard plotting libraries.

```
# add a column indicating the model
sims_df <- opt_sims %>% mutate(model = "Optimal")
policy_df <- opt_policy  %>% mutate(model = "Optimal")

# plot results as separate panels
plot_sims(sims_df) / ( plot_policy(policy_df) + plot_reward(sims_df))
```

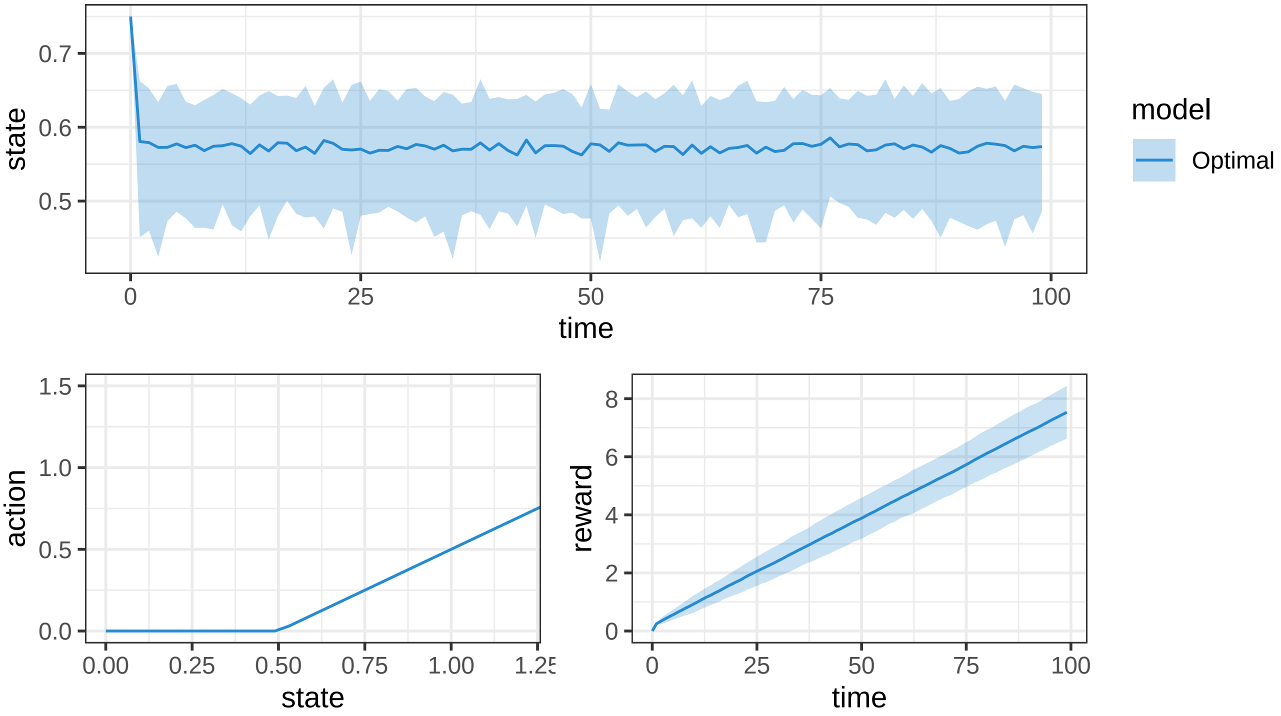


### 5.3 RL-based solutions

We will compare this optimal solution with results from the several different RL algorithms. Unlike the optimal solution, the RL methods never know the underlying growth function used by the simulation (or even if such a function actually exists). These methods merely seek to learn a strategy for setting harvest quotas which maximizes the cumulative reward they receive from the environment. At the heart of each deep RL algorithm is a neural network or a collection of neural networks. Model-free RL agents use these networks to approximate a policy function and/or a value function – see Appendix A for more detail here. Confusingly, the parameters of a RL algorithm that detail the overall learning process are called *hyperparameters* while the parameters of a RL algorithm that are learned during training are called parameters. For example, the number of layers in a neural network is a hyperparameter, but a weight in the neural net is referred to as a parameter. Before training an agent, we must first specify the hyperparameters; the parameters, meanwhile, are typically randomly initialized. Note that each algorithm may have different hyperparameters, so it is helpful to look at the algorithm's documentation to know what these hyperparameters are. `stable-baselines3` provides default values for all hyperparameters based on the original papers that introduced the corresponding algorithms.

For example, here we will use the Twin Delayed DDPG method (TD3) described in Fujimoto, Hoof, and Meger (2018). This algorithm is a successor of Deep Deterministic Policy Gradient (DDPG) method (Lillicrap et al. 2019), itself a policy-gradient-modification that extends the original Deep Q-Network (DQN) algorithm (Mnih et al. 2015) to continuous action spaces. We use this algorithm to train an agent that employs multi-layer perceptron (`MlpPolicy`) neural networks, with the default architecture of two 64-neuron layers.

```
env = gym$make("fishing-v1", sigma=0.1)
agent = sb3$TD3('MlpPolicy', env, seed = seed)
```

Training is the main computationally intensive process, which can take anywhere from a few minutes to many days, depending on the complexity of the environment, the neural network architecture and the number of training iterations budgeted. Therefore, we save the trained agent to disk, and only execute the training method (`learn`) if no previously saved agent is found:

```r
if(!file.exists("../python/cache/td3_untuned.zip")) {

  # Train the agent for a fixed number of timesteps
  agent$learn(total_timesteps=300000L)

  # Save our trained agent for future use
  agent$save("../python/cache/td3_untuned")

}
```

Note that while default hyperparameters provide a useful starting place (particularly when the environment has been suitably normalized, a best-practice we discuss below), better performance can almost always be achieved by *tuning* the hyperparameter selection. This is discussed further below. Having saved our trained agent to disk, we can then re-load this agent for evaluation or to continue training. Note that a copy of the trained agents are included in the corresponding GitHub repository.

```r
# load the trained agent from cache
agent = sb3$TD3$load("../python/cache/td3_untuned")
```

We can supply an observation to our trained agent and it will return its proposed action using the `predict` method. This is all we need to evaluate or employ the agent on a decision-making task. Recall that state space and action space in the fishing gym have been re-scaled to a (-1, 1) interval. Note that this is equivalent to a choice of appropriate units – we can re-scale the interval without loss of generality. This is often an important step in the design of an RL environment to facilitate successful training. Following the `gym` standard, the core methods such as `predict` and `step` operate on the re-scaled units, so it is necessary to first transform the original units into this re-scaled state space. For example, if we wish to start a simulation with a stock size of 0.75, we can use the helper method `get_state()`, to determine the corresponding value in the re-scaled state space.
Unlike `predict` and `step`, `get_state()` is not a standard method of all gym environments – typically a user must first inspect the state space of an environment and choose themselves how to re-scale their problem into that state space.

```r
## represent the initial state size in the 'rescaled' state space.
state = env$get_state( 0.75 )
state
```

```
## [1] -0.25
```

With an initial state in hand, we are ready to simulate management using our agent. The iteration is simple: we use the agent to predict what action we should take given the current state. Then, we take said action and examine the result to determine the future state. Because these methods return additional information as well, a little extra sub-setting is required in R:

```r
for(i in 1:10){

  out = agent$predict(state, deterministic=TRUE)
  action = out[[1]]
  result = env$step(action)
  state = result[[1]]

}
```

For convenience, `gym_fishing` defines the helper routine `simulate` to perform the above iteration `reps` number of times. The `simulate` method returns the state, action, and reward resulting from each time step of each replicate:

```r
agent_sims = env$simulate(agent, reps = 100L)
```

Because the agent typically attempts to retain the fish population near a specific value, simulations with well-trained agents will usually not explore the full range of possible states. To get a better idea of how

the agent behaves across the full state space, it is common to examine the policy function: to do this, we'll plot the action taken at every possible state. Some agents are non-deterministic, so we may want to use replicate draws at each state to get a better picture of the agent's behavior. Note that the `policyfn` method is another custom method and not part of the `gym` standard. The use of `policyfn` will not make sense for agents that consider the history of many previous states in selecting their action, such as agents which utilize recurrent neural network architectures like LSTMs (Bakker 2007).

```
agent_policy = env$policyfn(agent, reps = 5L)
```

```
# stack result simulations with those above and plot:
sims_df <- agent_sims %>%
  mutate(model = "TD3_untuned") %>%
  bind_rows(sims_df)
policy_df <- agent_policy  %>%
  mutate(model = "TD3_untuned")  %>%
  bind_rows(policy_df)

plot_sims(sims_df) / ( plot_policy(policy_df) + plot_reward(sims_df))
```

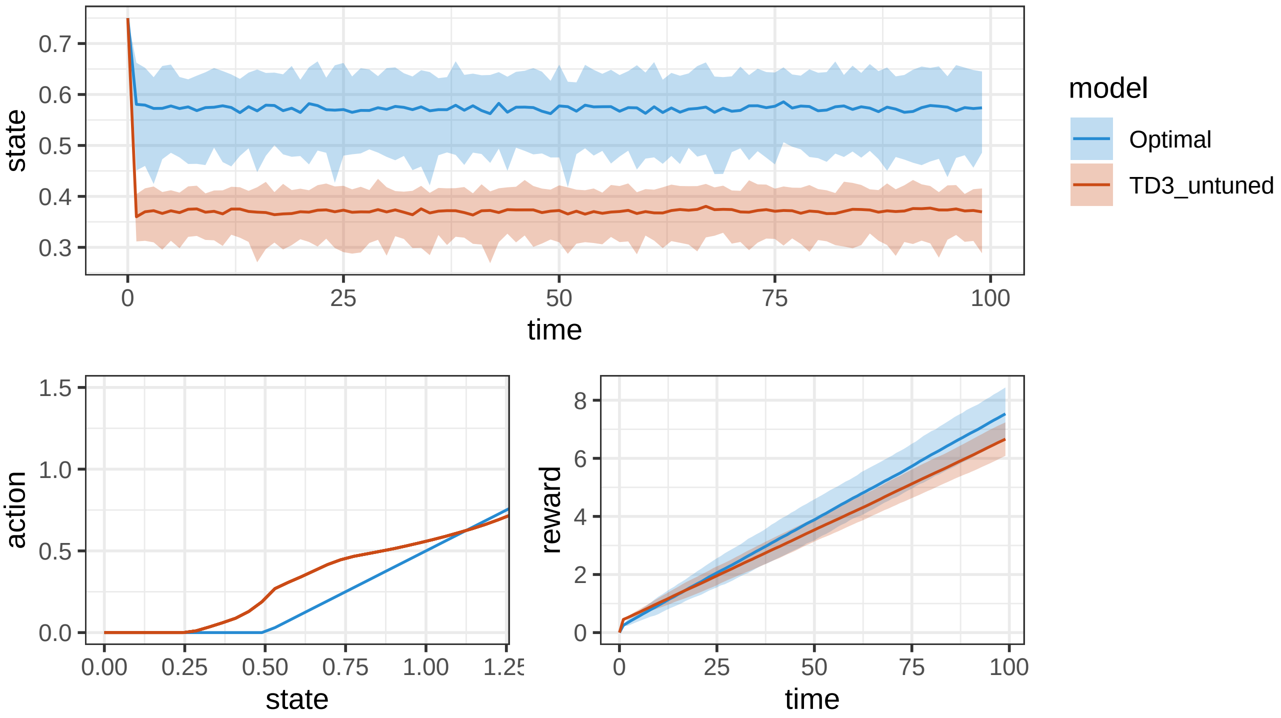


As we can see in the figure above, without hyperparameter tuning, our agent has found only a sub-optimal policy. The RL agent trained under an un-tuned TD3 algorithm here tends to over-harvest the fishery, resulting in an initially higher reward that grows steadily but more slowly than the optimal strategy. As discussed in the main text, training of Deep RL algorithms is subject to several sources of instability that can make it difficult or impossible to reproduce the same results from training with the same hyperparameters on different hardware or hardware drivers, even when controlling for random seed (Nagarajan, Warnell, and Stone 2019; Henderson et al. 2019). Consequently, users may not recover identical behavior when training under identical parameters. However, by using the cached neural network parameter weights of the trained agent, users should be able to reproduce the same agent behavior.

### 5.4 Tuning hyperparameters

By tuning the hyperparameters that control the training regime used by the TD3 algorithm, we are able to further improve upon on the performance of the RL agent. Tuning may be performed manually by adjusting hyperparameters based on mechanistic reasoning (e.g. larger action noise may improve exploration over exploitation, a larger neural network may better approximate a more complex policy). This search can also be automated using standard non-linear optimization techniques, adjusting hyperparameters to maximize the reward attained by the trained network. Using such an approach (see `https://github.com/boettiger-lab/conservation-agents`), we discover the following hyperparameters achieve better performance (see Fujimoto, Hoof, and Meger (2018) or Raffin et al. (2019) documentation for formal definitions of each hyperparameter) :

```
td3 = sb3$TD3('MlpPolicy',
              env,
              seed = 42L,
              gamma = 0.995,
              learning_rate = 0.0001355522450968401,
              batch_size = 128L,
              buffer_size = 10000L,
              train_freq = 128L,
              gradient_steps = 128L,
              action_noise = sb3$common$noise$NormalActionNoise(
                mean=np$zeros(1L),
                sigma= 0.6656948079225263 * np$ones(1L)),
              policy_kwargs = list(net_arch=c(400L, 300L)))
```

We train this new RL agent using its tuned hyperparameters, and saving the resulting trained agent as before:

```
if(!file.exists("../python/cache/td3_tuned.zip")){
  td3$learn(total_timesteps=300000L)
  td3$save("../python/cache/td3_tuned.zip")
}
```

Once our agent has been trained, we can again evaluate its performance across replicate simulations:

```
td3 <- sb3$TD3$load("../python/cache/td3_tuned.zip")

td3_sims = env$simulate(td3, reps = 100L)
td3_policy = env$policyfn(td3)
```

```
# stack result simulations with those above and plot:
sims_df <- td3_sims %>%
  mutate(model = "TD3") %>%
  bind_rows(sims_df)
policy_df <- td3_policy  %>%
  mutate(model = "TD3")  %>%
  bind_rows(policy_df)


plot_sims(sims_df) / ( plot_policy(policy_df) + plot_reward(sims_df))
```

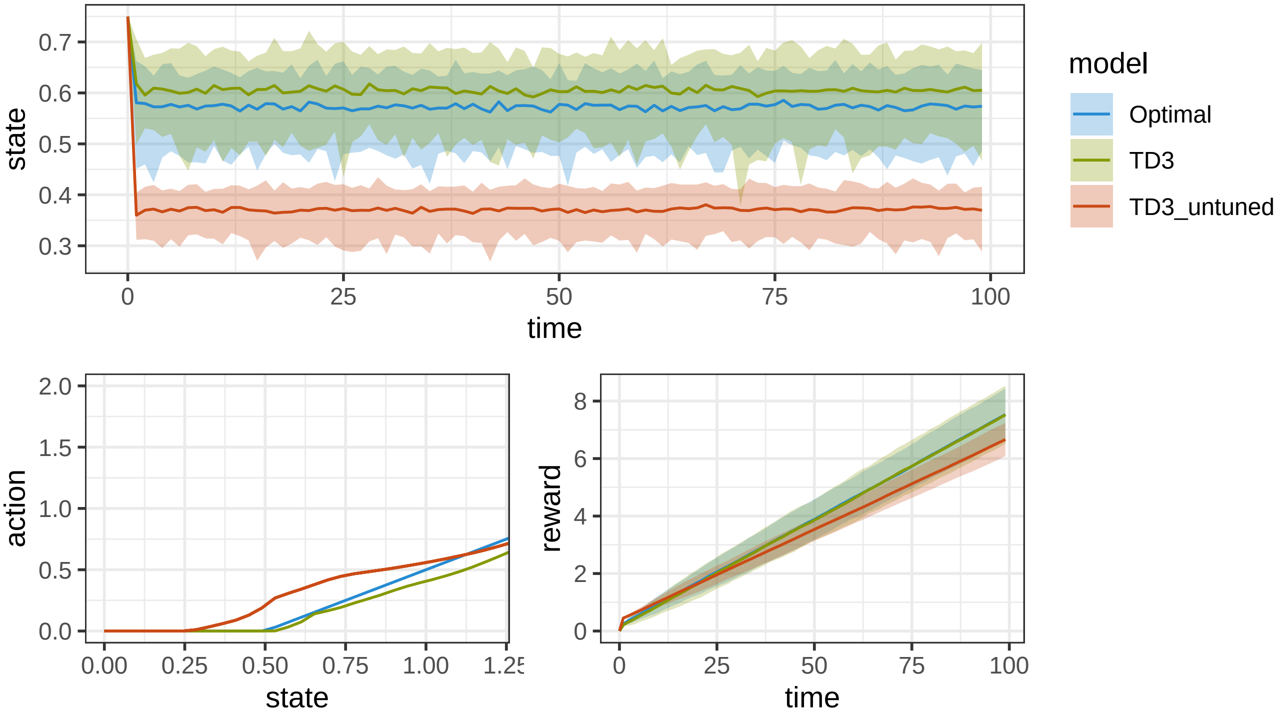


In this simple example, the RL tuned agent is able to achieve nearly-optimal performance (as defined by the reward conditions). Note that the largest deviations from the optimal policy occur at large stock sizes, at or above carrying capacity of the model. This pattern is not surprising, since these large stock values are least likely to be observed over the simulated episodes. For the same reason, that deviation contributes very little to the observed reward. Only by comparing average stock sizes directly can we see that the RL agent slightly under-harvests on average relative to the optimal policy. As noted in appendix C, careful design of the environment, such as re-scaling of state and action space, can also improve the ability of a Deep RL algorithm to find an acceptable policy without altering the substance of the challenge. Even so, our agent still had extensive time to train on this specific environment, a total of 300,000 timesteps.

## 6 Ecological tipping points

Our second example utilizes our `gym_conservation` to provide the necessary environment to simulate an ecosystem approaching a tipping point.

### 6.1 Tipping point model

The tipping point model is based on the consumer-resource model of May (1977), which creates alternative stable states, which we subject to log-normal environmental noise:

$$\mu_t = X_t + X_t r \left(1 - \frac{X_t}{K}\right) - \frac{a_t X_t^q}{X_t^q + b^q}$$

$$X_{t+1} \sim \text{lognormal}(\mu_t, \sigma)$$

where we take $r = 0.7$, $K = 1.2$, $q = 3$, $b = 0.15$, $a_0 = 0.19$ and $\sigma = 0.2$ Slow change over time in the parameter $a_t$ represents a process of environmental degradation, modeled as a constant increment $a_{t+1} = a_t + \alpha$, where we will take $\alpha = 0.001$. This model supports the dynamics of a fold bifurcation, widely used to model critical transitions in both theory and empirical manipulation in systems from microbes (Dai et al. 2012) to lakes (Carpenter et al. 2011) to the planet biosphere (Barnosky et al. 2012).

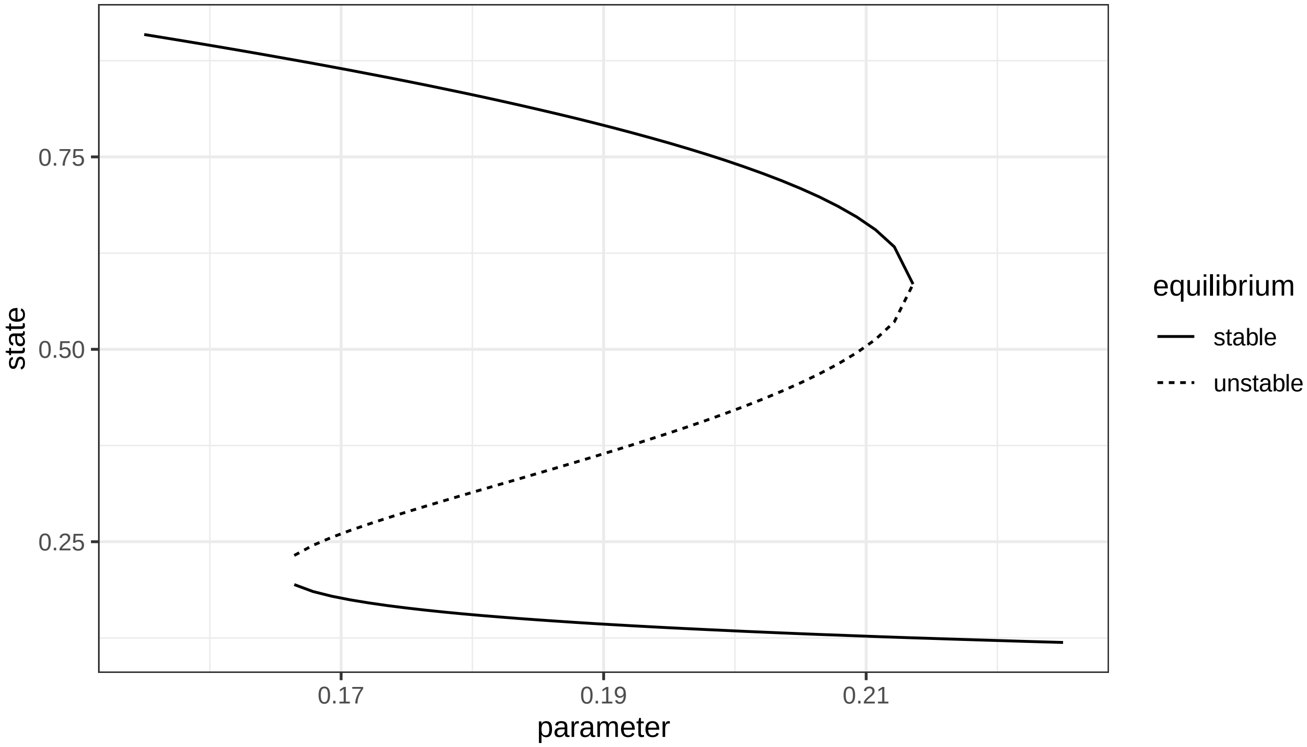


Figure 1: Bifurcation diagram for tipping point scenario. The ecosystem begins in the desirable 'high' state under an evironmental parameter (e.g. global mean temperature, arbitrary units) of 0.19. In the absence of conservation action, the environment worsens (e.g. rising mean temperature) as the parameter increases. This results in only a slow degredation of the stable state, until the parameter crosses the tipping point threshold at about 0.215, where the upper stable branch is anihilated in a fold bifurcation and the system rapidly transitions to lower stable branch, around state of 0.1. Recovery to the upper branch requires a much greater conservation investment, reducing the parameter all the way to 0.165 where the reverse bifurcation will carry it back to the upper stable branch.

```
bifur_df = read_csv("../manuscript/figs/bifur.csv", col_types = "dccd")
bifur_df %>%
  ggplot(aes(parameter, state, lty=equilibrium, group = group)) +
  geom_line()
```

We assume the benefit provided by the ecosystem state is assumed to be directly proportional to the state itself, $bx_t$.
We further assume that each year the manager has the option to slow or reverse the environmental degradation by taking action $A_t$, such that under management, the resulting environment in the next time step is given by

$$a_{t+1} = a_t + \alpha - A_t$$

We assume the cost associated with that action to be proportional to the square of the action, such that large actions are proportionally more costly than small ones. Consequently, the utility at time $t$ is given by the sum of costs and benefits:

$$U(X_t, A_t) = bX_t - cA_t^2$$

where we will take $b = 1$ and $c = 1$.
Our implementation in `gym_conservation` allows the user to consider alternative parameter choices, alternative models for the ecological dynamics, and alternate types of actions, such as manipulating the ecosystem

state directly rather than manipulating the environmental parameter. For some such scenarios the optimal solution is known or can be determined by stochastic dynamic programming, while for others, including the scenario of focus here, the optimal solution is unknown.

```
# Python users see python/conservation_TD3.py
env = gym$make("conservation-v6")

noise_std = 0.4805935357322933
OU = sb3$common$noise$OrnsteinUhlenbeckActionNoise
action_noise = OU(mean = np$zeros(1L),  sigma = noise_std * np$ones(1L))

model = sb3$TD3('MlpPolicy',
            env,
            verbose = 0,
            seed = 42L,
            "gamma"= 0.995,
            "learning_rate"=  8.315382409902049e-05,
            "batch_size"= 512L,
            "buffer_size"= 10000L,
            "train_freq"= 1000L,
            "gradient_steps"= 1000L,
            "action_noise"= action_noise,
            "policy_kwargs"= list("net_arch"= c(64L,64L)))
```

As before, we train the agent unless a cached version of the trained agent is already available:

```
if(!file.exists("../python/cache/td3-conservation.zip")){

  model$learn(total_timesteps=3000000L)
  model$save("../python/cache/td3-conservation")

}
```

```
model = sb3$TD3$load("../python/cache/td3-conservation")
TD3_sims = env$simulate(model, reps = 100L) %>% mutate(model = "TD3")
TD3_policy = env$policyfn(model, reps = 1L)  %>% mutate(model = "TD3")
```

In general, the optimal solution depends on the ecological dynamics, the benefit of the ecosystem services and the costs associated with a management response. Because the tipping point problem is non-autonomous, we cannot solve for the optimal policy even given the model and objective (utility) function using Markov Decision Process methods. However, a simple heuristic solution provides a reasonable starting point for comparison.

As discussed in the main text, we have no existing optimal solution to the tipping point problem, and so rely on a common heuristic strategy instead: select a fixed level of conservation investment that is sufficient to counter-balance any further side towards the tipping point, preserving it in its current state. This is implemented using the `fixed_action` method provided in our `gym_conservation` module, which also implements other heuristic models, including a human agent which requires interactive input to select the action each year.

```
# Simulate under the steady-state solution (given the model)
K = 1.5
alpha = 0.001
opt = gym_conservation$models$fixed_action(env, fixed_action = alpha * 100 * 2 * K )
opt_sims = env$simulate(opt, reps = 100L) %>% mutate(model="steady-state")
opt_policy = env$policyfn(opt) %>% mutate(model="steady-state")
```

We gather together the results under the RL agent and steady-state policy as before,

```
sims_df = bind_rows(TD3_sims, opt_sims)
policy_df = bind_rows(TD3_policy, opt_policy)
```

The resulting three data frames contain the necessary data for each of the subplots in figure 3 of the main text.

```
write_csv(sims_df, "../manuscript/figs/tipping_sims_df.csv")
write_csv(policy_df, "../manuscript/figs/tipping_policy_df.csv")
```

```
plot_sims(sims_df) / ( plot_policy(policy_df) + plot_reward(sims_df))
```

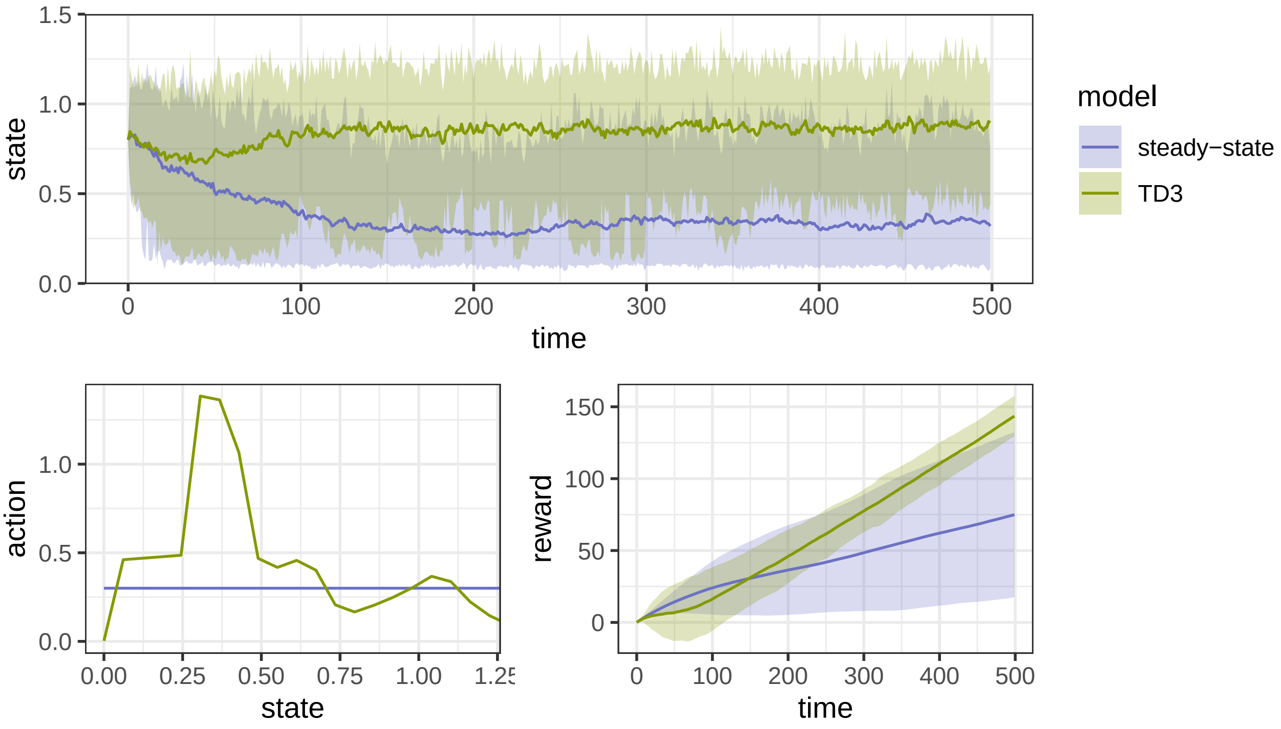


### 6.2 Rescues: individual simulation trajectories

Because it is difficult to get a feel for the dynamics of individual replicate simulations from ensemble statistics, we select a few example trajectories to examine directly. Of the 100 replicate simulations, we pick 4 examples that dip below a state value of 0.2 for over 15 consecutive timesteps, indicating a transition into the lower basin of attraction. Comparing the dynamics under the rule of thumb steady-state strategy to that of the RL-trained agent, it is clear that the RL agent does a better job at both avoiding tipping points and promoting the recovery of those selected trajectories that cross into the lower attractor.

```
# Some individual replicates, for comparison

## First 4 of the TD3 reps falling below .2 for more than 15 steps
is_low = sims_df %>%
  filter(model == "TD3") %>%
  group_by(rep, model) %>%
  summarize(low = sum(state < .2) > 10) %>%
  filter(low) %>% head(6)

## First 4 such cases:
sims_df %>% inner_join(is_low) %>%
```

```
  ggplot(aes(time, state,  col=model, group=interaction(model, rep))) +
  geom_line(show.legend = FALSE) + facet_wrap(~rep)
```

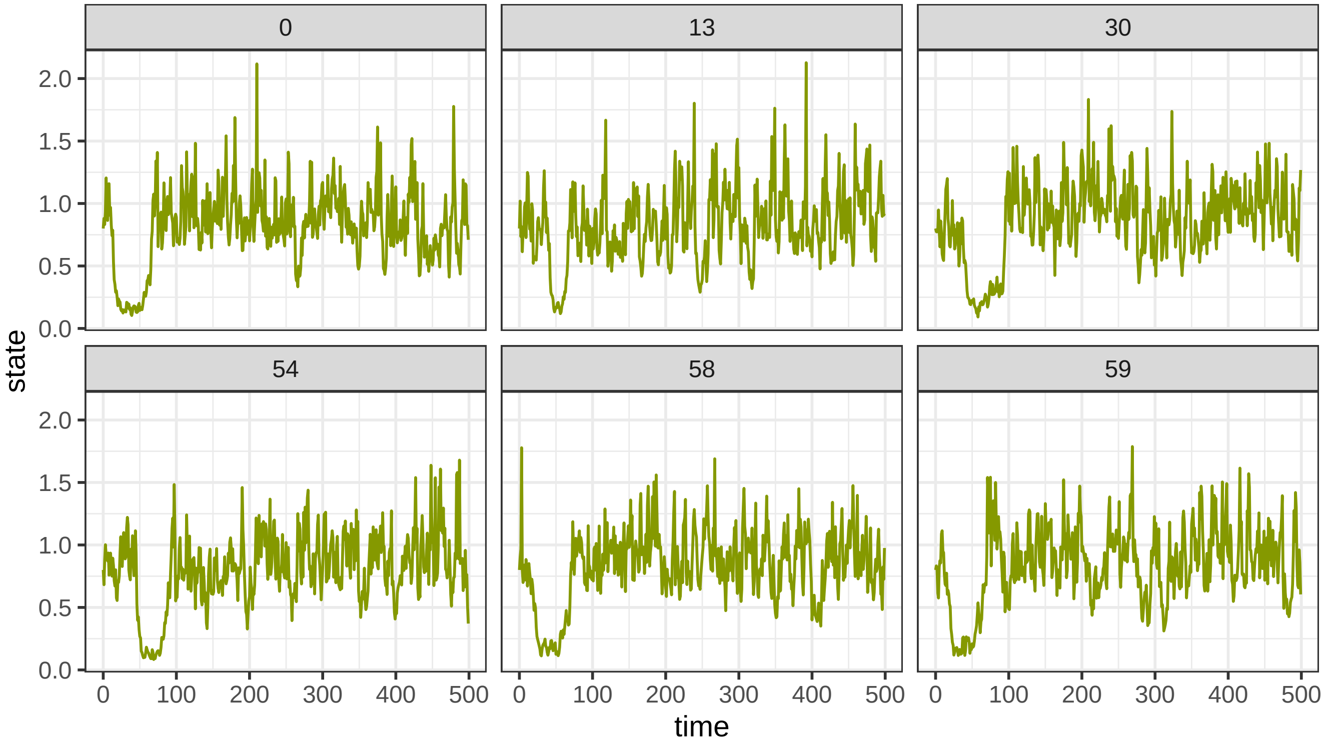


```
# Some individual replicates, for comparison
is_low = sims_df %>% filter(model == "steady-state") %>%
  group_by(rep, model) %>% summarize(low = sum(state < .2) > 10) %>%
  filter(low) %>% head(6)
sims_df %>% inner_join(is_low) %>%
  ggplot(aes(time, state, col=model, group=interaction(model, rep))) +
  geom_line(show.legend = FALSE) + facet_wrap(~rep)
```

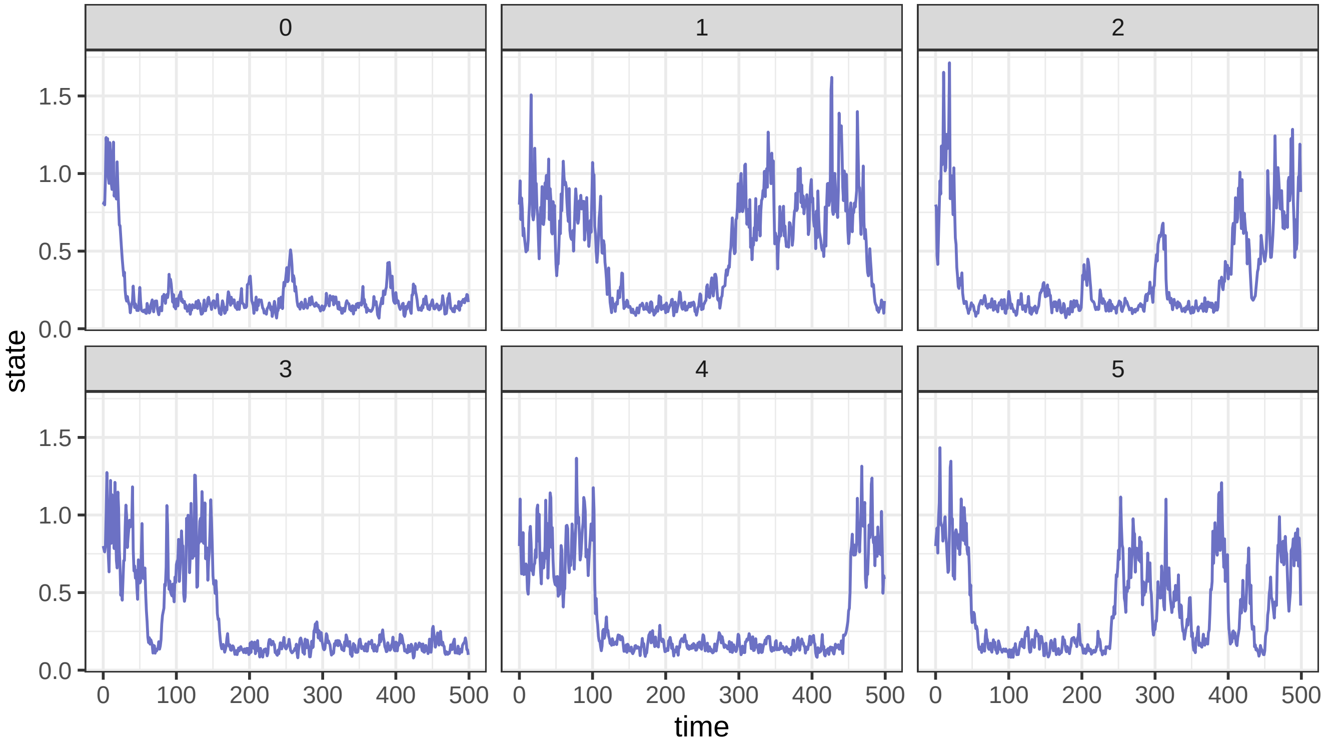
0
1
2
3
4
5
state
0.0
0.5
1.0
1.5
time
0
100
200
300
400
500

## References

Achiam, Joshua. 2018. "Spinning Up in Deep Reinforcement Learning."

Bakker, Bram. 2007. "Reinforcement Learning by Backpropagation Through an LSTM Model/Critic." In *2007 IEEE International Symposium on Approximate Dynamic Programming and Reinforcement Learning*, 127–34. https://doi.org/10.1109/ADPRL.2007.368179.

Barnosky, Anthony D., Elizabeth A. Hadly, Jordi Bascompte, Eric L. Berlow, James H. Brown, Mikael Fortelius, Wayne M. Getz, et al. 2012. "Approaching a State Shift in Earth's Biosphere." *Nature* 486 (7401): 52–58. https://doi.org/10.1038/nature11018.

Carpenter, Stephen R, J. J. Cole, Michael L Pace, Ryan D. Batt, William A Brock, Timothy J. Cline, J. Coloso, et al. 2011. "Early Warnings of Regime Shifts: A Whole-Ecosystem Experiment." *Science (New York, N.Y.)* 1079 (April). https://doi.org/10.1126/science.1203672.

Dai, Lei, Daan Vorselen, Kirill S Korolev, and J. Gore. 2012. "Generic Indicators for Loss of Resilience Before a Tipping Point Leading to Population Collapse." *Science (New York, N.Y.)* 336 (6085): 1175–77. https://doi.org/10.1126/science.1219805.

Fujimoto, Scott, Herke van Hoof, and David Meger. 2018. "Addressing Function Approximation Error in Actor-Critic Methods." *arXiv:1802.09477 [Cs, Stat]*, October. http://arxiv.org/abs/1802.09477.

Guadarrama, Sergio, Anoop Korattikara, Oscar Ramirez, Pablo Castro, Ethan Holly, Sam Fishman, Ke Wang, et al. 2018. "TF-Agents: A Library for Reinforcement Learning in TensorFlow." https://github.com/tensorflow/agents. https://github.com/tensorflow/agents.

Henderson, Peter, Riashat Islam, Philip Bachman, Joelle Pineau, Doina Precup, and David Meger. 2019. "Deep Reinforcement Learning That Matters." *arXiv:1709.06560 [Cs, Stat]*, January. http://arxiv.org/abs/1709.06560.

Hill, Ashley, Antonin Raffin, Maximilian Ernestus, Adam Gleave, Anssi Kanervisto, Rene Traore, Prafulla Dhariwal, et al. 2018. "Stable Baselines." *GitHub Repository*. https://github.com/hill-a/stable-baselines; GitHub.

Lillicrap, Timothy P., Jonathan J. Hunt, Alexander Pritzel, Nicolas Heess, Tom Erez, Yuval Tassa, David Silver, and Daan Wierstra. 2019. "Continuous Control with Deep Reinforcement Learning." *arXiv:1509.02971 [Cs, Stat]*, July. http://arxiv.org/abs/1509.02971.

May, Robert M. 1977. "Thresholds and Breakpoints in Ecosystems with a Multiplicity of Stable States." *Nature* 269 (5628): 471–77. https://doi.org/10.1038/269471a0.

Mnih, Volodymyr, Koray Kavukcuoglu, David Silver, Andrei A. Rusu, Joel Veness, Marc G. Bellemare, Alex Graves, et al. 2015. "Human-Level Control Through Deep Reinforcement Learning." *Nature* 518 (7540): 529–33. https://doi.org/10.1038/nature14236.

Nagarajan, Prabhat, Garrett Warnell, and Peter Stone. 2019. "Deterministic Implementations for Reproducibility in Deep Reinforcement Learning." *arXiv:1809.05676 [Cs]*, June. http://arxiv.org/abs/1809.05676.

Paszke, Adam, Sam Gross, Francisco Massa, Adam Lerer, James Bradbury, Gregory Chanan, Trevor Killeen, et al. 2019. "PyTorch: An Imperative Style, High-Performance Deep Learning Library." In *Advances in Neural Information Processing Systems 32*, edited by H. Wallach, H. Larochelle, A. Beygelzimer, F. dAlché-Buc, E. Fox, and R. Garnett, 8024–35. Curran Associates, Inc. http://papers.neurips.cc/paper/9015-pytorch-an-imperative-style-high-performance-deep-learning-library.pdf.

Plappert, Matthias. 2016. "Keras-Rl." *GitHub Repository*. https://github.com/keras-rl/keras-rl; GitHub.

Raffin, Antonin, Ashley Hill, Maximilian Ernestus, Adam Gleave, Anssi Kanervisto, and Noah Dormann. 2019. "Stable Baselines3." *GitHub Repository*. https://github.com/DLR-RM/stable-baselines3; GitHub.

Reed, William J. 1979. "Optimal escapement levels in stochastic and deterministic harvesting models." *Journal of Environmental Economics and Management* 6 (4): 350–63. https://doi.org/10.1016/0095-0696(79)90014-7.

"Reticulate." 2018. *GitHub Repository*. https://github.com/rstudio/reticulate; GitHub.

"Rocker." 2018. *GitHub Repository.* `https://github.com/rocker-org/rocker`; GitHub.

Schaefer, Milner B. 1954. "Some aspects of the dynamics of populations important to the management of the commercial marine fisheries." *Bulletin of the Inter-American Tropical Tuna Commission* 1 (2): 27–56. `https://doi.org/10.1007/BF02464432`.

"Tensorflow." 2018. *GitHub Repository.* `https://github.com/tensorflow/tensorflow`; GitHub.
