# Supplementary material for: Deep Reinforcement Learning for Conservation Decisions
Source: arXiv:2106.08272 source file (2021-06-15)
Supplement: Supplementary file 3 [file appendix-C-environments.pdf]

# Appendix C: Building Environments for Deep Reinforcement Learning

A Preprint

**Marcus Lapeyrolerie**
Department of Environmental Science, Policy, and Management
University of California, Berkeley
Berkeley, California

**Melissa Chapman**
Department of Environmental Science, Policy, and Management
University of California, Berkeley
Berkeley, California

**Kari Norman**
Department of Environmental Science, Policy, and Management
University of California, Berkeley
Berkeley, California

**Carl Boettiger**
Department of Environmental Science, Policy, and Management
University of California, Berkeley
Berkeley, California
cboettig@berkeley.edu

June 13, 2021

## 1 Defining an Environment

In Deep Reinforcement Learning (DRL), an *environment* is a mathematical model, computer simulation, or real world situation with which the agent interacts. Defining an *environment* requires 5 components:

1. Describe the states defining the environment
2. Describe the possible actions available to the agent
3. Update the environment's internal *state* in response to the *action* of the *agent*
4. Provide the agent with an *observation* of the new state
5. Provide the agent with a *reward* based on the environment's state and the agent's action.

Mathematically, these actions can be expressed as functions: a *step function* $f$ providing the new state, $s_{t+1}$ given the current state $s_t$ and the agent's most recent action $a_t$:

$$s_{t+1} = f(s_t, a_t),$$

an observation function (sometimes called the 'emission' function, $E$) giving the observed state as a function of the current state and possibly also the action (i.e. different actions could potentially influence the accuracy of the observation):

$$o_{t+1} = E(s_t, a_t)$$

and a reward $r_t$ given by a utility function $U$ of the current state and action,

$$r_t = U(s_t, a_t)$$

This corresponds to the formal definition of a Partially Observed Markov Decision Process (POMDP), see main text.

## 2 A Minimal Example based on Fishing Quotas

For example, consider the fishing quota problem.

1. The state space is defined as the current total biomass of the fish stock, that is, any non-negative real number. For simplicity, we might restrict our representation of the state space to a sufficiently large value unlikely to be reached, such as twice the carrying capacity, $s_t \in [0, 2K]$. Note that in a more general problem, the state space could be a vector of real values, e.g. giving the biomass of different age classes and/or different interacting species.
2. For simplicity, we assume the harvest quota can reach any possible state value, $a_t \in [0, 2K]$.
3. The step function is given by the Gordon-Schaefer model,

$$s_{t+1} = s_t + r s_t \left(1 - \frac{s_t}{K}\right) - a_t,$$

(In `gym_fishing-v1` an optional stochastic growth term is also included).

4. observations are made without error, $o_t = s_t$,
5. and the utility is given by the amount harvested (i.e. the harvest quota, so long as it does not exceed the total stock):

$$r_t = \min(a_t, x_t)$$

## 3 A Minimal Example in Python

In order to interface with existing frameworks for implementing deep RL, it is convenient to express these mathematical functions as computational functions. By following the specification defined in Brockman et al. (2016), we can create a python module, often referred to as a "gym," that expresses the five elements in standardized form.

A minimal `gym` object inherits from the `gym.Env` class, and provides a `step()` method and `reset()` method:

```
import gym
import numpy as np
from gym import spaces

class FishingEnv(gym.Env):

    def __init__(self, r = 0.3, K = 1, s0 = 0.75, Tmax=100):

        # parameters
        self.K = K
        self.r = r
        self.s0 = s0
        self.Tmax = Tmax

        # Initial conditions
        self.state = self.s0
        self.year = 1

        # State and action space
        self.observation_space = spaces.Box(0., 2.*self.K)
        self.action_space = spaces.Box(0., 2.*self.K)


    def step(self, action):

        # Step function
        self.state = self.state + self.r * self.state (1 - self.state / self.K) - action

        # Utility function
        reward = min(quota, self.state)

        # Observation function
        observed = self.state

        # End conditions
        self.year = self.year + 1
        done = bool(self.year > self.Tmax)

        # Return observation, reward, end condition and optional info
        return observed, reward, done, {}

    def reset(self):
        self.state = self.s0
        self.year = 0
        return self.state
```

In practice, an environment may include additional logic for rendering information about it's current states as output. Effective environments may often work in a transformed variable space, for example, `gym_fishing` maps the space $[0, 2K]$ into the space $[-1, 1]$, which significantly improves agent performance. Other features, such as 32 bit precision numeric values for state and action spaces, can also improve agent performance with GPU-based computation.

Function inheritance provides a natural way to express many variations of a gym, such as alternate step functions, utility functions, or even alternate action and state spaces. Standard python module structure facilitates installing and loading a gym. Unit testing and continuous integration provide a reliable mechanism to ensure the gym is working as expected. The `gym_fishing` repository, `https://github.com/boettiger-lab/gym_fishing` illustrates all of these elements.

## References

Brockman, Greg, Vicki Cheung, Ludwig Pettersson, Jonas Schneider, John Schulman, Jie Tang, and Wojciech Zaremba. 2016. "OpenAI Gym." *arXiv:1606.01540 [Cs]*, June. http://arxiv.org/abs/1606.01540.
