# Supplementary material for: Deep Reinforcement Learning for Conservation Decisions
Source: arXiv:2106.08272 source file (2021-06-15)
Supplement: Supplementary file 4 [file appendix-D-data.pdf]

# Appendix D: Accessing Empirical Data for Management Comparison

A Preprint

**Marcus Lapeyrolerie**
Department of Environmental Science, Policy, and Management
University of California, Berkeley
Berkeley, California

**Melissa Chapman**
Department of Environmental Science, Policy, and Management
University of California, Berkeley
Berkeley, California

**Kari Norman**
Department of Environmental Science, Policy, and Management
University of California, Berkeley
Berkeley, California

**Carl Boettiger**
Department of Environmental Science, Policy, and Management
University of California, Berkeley
Berkeley, California
cboettig@berkeley.edu

June 13, 2021

This appendix provides reproducible code used to access and clean data from the R.A. Myers Legacy Stock Assessment Database used in for empirical comparison in the hindcasts shown in the main text.

```
# R dependencies
library(tidyverse)
library(patchwork)
library(reticulate)

## Python dependencies loaded via R
sb3      = import("stable_baselines3")
torch    = import("torch")
gym      = import("gym")
gym_fishing = import("gym_fishing")
gym_conservation = import("gym_conservation")
```

```r
source("../R/plotting-helpers.R")
```

Access data from the RAM Legacy Stock Assessment Database. (2020). Version v4.491 [Data set]. Zenodo. http://doi.org/10.5281/zenodo.3676088. Note that DOIs resolve only to HTML landing pages.
For programmatic access to the data, we resolve content by it's content hash instead:

```r
library(contentid)
ramzip <- resolve("hash://md5/fac27d8b7876df29afaeadcd7f5a3b77")
unzip(ramzip, exdir = "ramlegacy")
load("ramlegacy/RAMLDB v4.491/DB Files With Assessment Data/R Data/DBdata[asmt][v4.491].RData")
```

Relevant data is stored across several tables, following relational database practices.
Before analysis we join these tables by shared primary key:

```r
ramlegacy <-
  timeseries_values_views %>%
  select(stockid, stocklong, year, SSB, TC) %>%
  left_join(stock) %>%
  left_join(area) %>%
  select(stockid, scientificname,
         commonname, areaname, country, year,
         SSB, TC) %>%
  left_join(timeseries_units_views %>%
              rename(TC_units = TC, SSB_units = SSB)) %>%
  select(scientificname, commonname,
         stockid, areaname, country, year,
         SSB, TC, SSB_units, TC_units)
```

Let's filter out missing data, non-matching units, and obvious reporting errors (catch exceeding total spawning biomass), then we re-scale each series into the 0,1 by appropriate choice of units. We store the processed data locally for future use.

```r
stock_ids <- c("ARGHAKENARG")

fish <- ramlegacy %>%
  filter(stockid %in% stock_ids) %>%
  filter(!is.na(SSB), !is.na(TC)) %>%
  filter(SSB_units == "MT", TC_units=="MT") %>%
  filter(SSB > TC) %>%
  select(-SSB_units, -TC_units) %>%
  group_by(stockid) %>%
  mutate(scaled_catch = TC / max(SSB),
         scaled_biomass = SSB / max(SSB))

hake <- fish  %>% filter(commonname=="Argentine hake")

hake %>% ggplot(aes(year, scaled_biomass)) + geom_point() + geom_line(aes(year, scaled_catch))
```

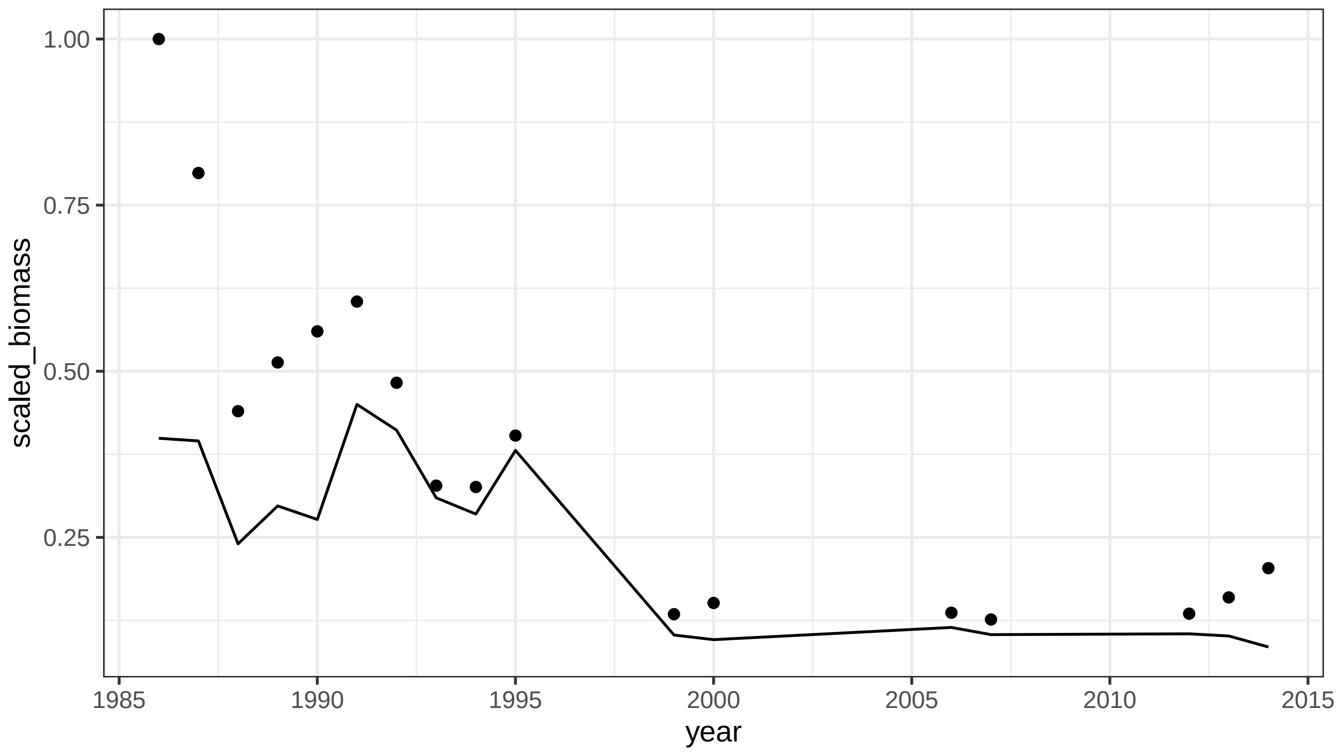


```
write_csv(hake, "../data/hake.csv")
```

### 0.1 Applying an RL agent to real data

We use historical data from Argentine Hake to illustrate how an RL agent might be applied in practice. Historical biomass and catch data for Argentine Hake can be found in the R.A. Myers Legacy Stock Assessment Database (RAM Legacy Stock Assessment Database 2020; Ricard et al. 2012). Here, we load a local copy of the stock assessment for the Argentine Hake from 1986 to 2000. (Annotated code for data cleaning can be found in Appendix D).

```
hake = read_csv("../data/hake.csv")
td3 = sb3$TD3$load("../python/cache/td3_tuned.zip")
env = gym$make("fishing-v1")
```

For each year in the data, we compare the historical harvest to the quota that would have been recommended by the TD3-based deep RL agent we trained in Appendix B. To utilize our RL agent to set a quota for the stock, we only have to map the observed biomass estimates and historical harvests into the re-scaled state space of the environment. Recall that the `gym_fishing` environment includes helper function `get_state()` to turn observed biomass to the state-space units used in the gym.

```
# Initial states
x0 = hake[[1, "scaled_biomass"]]
agent_state = agent_action = numeric(15)
agent_state[1] = x0
agent_action[1] = NA
N <- dim(hake)[1]
# `env` is used only to translate between original units and transformed space
# Represent the initial stock size in the 'rescaled' state space:
state = env$get_state(x0)
for(i in 1:N){

  # The RL agent recommends a Quota based on current state
```

```
  out = td3$predict(state)
  action = out[[1]]

  # We record state and proposed quota (in the original units)
  agent_state[i] = env$get_fish_population(state)
  agent_action[i] = env$get_quota(action)

  # Use historical data to determine the next state
  state = env$get_state(hake$scaled_biomass[i+1])
}
```

Plot the results:

```
harvest = bind_rows(
  tibble(year = hake$year, harvest = agent_action, model = "TD3"),
  tibble(year = hake$year, harvest = hake$scaled_catch, model = "historical")
)
stock <-  tibble(year =hake$year, biomass = hake$scaled_biomass, model = "historical")


write_csv(harvest, "../manuscript/figs/historical_harvest.csv")
write_csv(stock, "../manuscript/figs/historical_stock.csv")

top_panel <- ggplot(stock, aes(year, biomass, col=model)) + geom_line(lty=2) +
  theme(axis.title.x=element_blank(),
        axis.text.x=element_blank(),
        axis.ticks.x=element_blank())
bottom_panel <- ggplot(harvest, aes(year, harvest, col=model)) +
  geom_line() + geom_point()

top_panel / bottom_panel
```

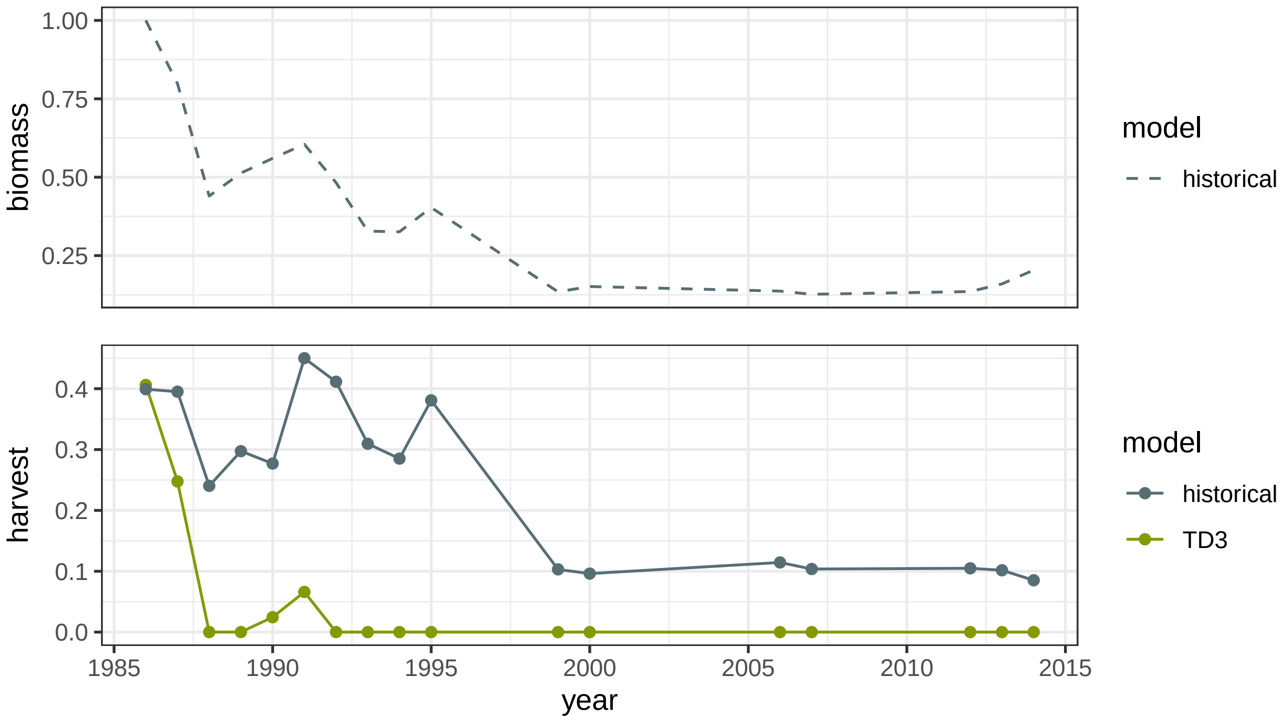

The Argentine hake biomass exhibited a steep decline between 1986 and 2014 as shown by the stock assessment estimates. Over that time, historical harvests showed some decline in step with the declining biomass. By contrast, for each of the historically observed biomass estimates the RL agent would have proposed much steeper cuts to the biomass quota which may have avoided the continued loss of biomass and eventual decline in harvest as well. This result should not be over-interpreted. Without being able to replay history, we have no way of truly knowing if the RL agent would have managed this stock better. While this example shows that it is in principle very straightforward to utilize a trained RL agent to recommend real harvest quotas, we must bear in mind that the agent is only as good as the environments on which it was trained. In practice, the RL agent would have to first be trained and evaluated on much more realistic environments than only the `fishing-v1` gym illustrated here.

RAM Legacy Stock Assessment Database. 2020. "RAM Legacy Stock Assessment Database V4.491." https://doi.org/10.5281/zenodo.3676088.

Ricard, Daniel, Cóilín Minto, Olaf P. Jensen, and Julia K. Baum. 2012. "Examining the Knowledge Base and Status of Commercially Exploited Marine Species with the RAM Legacy Stock Assessment Database." *Fish and Fisheries* 13 (4): 380–98. https://doi.org/10.1111/j.1467-2979.2011.00435.x.
